# Supplementary material for: IRS: An Incentive-compatible Reward Scheme for Algorand
Source: arXiv:2302.11178 source file (2023-02-22)
Supplement: Supplementary file 1 [file 12-appendix-background.tex]

\section{Additional Background}
\label{sec:background}

In this section, we provide some additional background materials including the common communication and adversary models, the consensus problem, proof of work and the finality of consensus protocols in blockchains.

\subsection{Communication Model}
In distributed systems, the underlying network usually suffers from uncertainty such that the messages could be delayed for some period.
The communication model defines the limit of such message delays.

There are three common communication models in distributed system literature: the Synchronous model, the Asynchronous model, and the Partially Synchronous model.
The following are the assumptions made for each model:

\begin{itemize}
    \item \textbf{Synchronous Model}: Any message sent will be received within a known time bound $t^\prime$.
    \item \textbf{Asynchronous Model}: Any message sent will be received within an unknown time bound.
    \item \textbf{Partially Synchronous Model} \cite{DLS1988}: Any message sent at time $t$ will be received within $t^\prime + max(t, GST)$ where $GST$ (Global Stabilization Time) is unknown.
\end{itemize}

One way to reason about the Partially Synchronous model is that the communication is asynchronous before GST and becomes synchronous after that.

\subsection{Adversary Model}
The nodes in a distributed system may suffer from some kinds of failures.
For example, a power shortage may cause a node to crash and a software bug could lead to undefined behaviour from the nodes.
Moreover, a malicious attacker may take full control of some nodes and make the nodes behave arbitrarily.
Theses failures are usually captured by assuming the existence of an adversary which can corrupt $f$ out of $n$ nodes in the system.

The adversaries are usually classified by the types of failure it can inflict on the corrupted nodes.
There are three common kinds of failure in distributed systems \cite{DLS1988}:

\begin{itemize}
    \item \textbf{Crash Failure}: The corrupted nodes stop sending or receiving any messages.
    \item \textbf{Omission Failure}: The corrupted nodes fail to send or receive messages when they should.
    \item \textbf{Byzantine Failure} \cite{LSP1982}: The corrupted nodes could send erroneous messages.
\end{itemize}

Note that the Byzantine failure is a superclass of the crash failure and the omission failure since a Byzantine node can pretend to be a one of these types.
There are many other failures but most of them can be subsumed by the Byzantine failure.
In a permissionless setting where everyone can join and leave the system at any time, such as Bitcoin \cite{Nakamoto2008}, the protocols designers usually focus on the Byzantine failure since it is the most general failure mode. In addition, malicious users can join the system and it is hard to predict what they will do.

Another important assumption about the adversary is the inability to break the cryptographic primitives used in the distributed systems.
Distributed systems usually assume a public key infrastructure (PKI) where each node has a public-private key pair $(pk, sk)$.
When a node wants to send a message $m$ to other nodes, it should send the signed version of the message $m_{sk}$ instead.
Other nodes can verify the signature using the sender's public key $pk$.
Many consensus protocols \cite{CL1999,GAG+2019,YMR+2019,GHM+2017} are based on the assumption that the adversary cannot forge the signature of correct nodes.
This prevents impossibility results caused by the issue where the adversary can simulate correct nodes \cite{FLM1985}.

\subsection{The Consensus Problem}
The consensus problem is one of the fundamental problems in distributed systems like blockchains.
It occurs when multiple nodes in the system need to make an agreement on a value.
In blockchains, the nodes in the system want to reach an agreement on the order and the content of the blocks, which contains an ordered set of transactions.
The formal definition of the consensus problem is defined as the following:

\begin{quote}
In a system with $n$ nodes indexed by $1, \dots, n$, there are $f$ out of $n$ nodes with failures.
Each node $i$ has an input value $v_i \in V$.
The nodes must decide a value among these inputs such that the following properties are satisfied \cite{DLS1988}:
\end{quote}

\begin{itemize}
    \item \textbf{Safety}: If a correct node decides a value $v$, all other correct nodes decide on the same value $v$. The decided value $v$ should satisfy the application-specific validity conditions.
    \item \textbf{Liveness}: All the correct nodes will eventually decide a value $v$.
\end{itemize}

A seminal work \cite{FLP1985} from Fischer, Lynch and Paterson proved that it is impossible to satisfy both properties under asynchronous communication model when there exists an adversary who can only crash one of the nodes.
However, as noted in the paper \cite{FLP1985}, this does not mean the consensus problem is not solvable under asynchronous network models; rather, the impossibility results indicate that more refined models or less strict requirements on the solutions are needed.
There are mainly two possible workarounds to circumvent the impossibility result.
The first method is by finding a middle ground between the synchronous model and the asynchronous model, such as the partially synchronous model introduced by \cite{DLS1988}.
Another method is to lighten the constraint on the liveness property by randomization such that all the correct nodes eventually decide a value $v$ with probability $1$ \cite{Ben-Or1983,BT1983,Bracha1984}.

The solutions to the consensus problem, usually called consensus protocols, are said to be $t$-resilient if they can tolerate up to $t$ faulty nodes.
The maximum number of corrupted nodes a consensus protocol can tolerate is called the optimal resilience of the protocol.
As shown in table \ref{table:optimal-resilience}, it has been proved in \cite{DLS1988,BT1983} that the optimal resilience of any asynchronous or semi-synchronous Byzantine consensus protocols is $\lfloor \frac{n-1}{3} \rfloor$ where $n$ is the total number of nodes.
If we assume the communication is synchronous, then the optimal resilience is increased to $\lfloor \frac{n-1}{2} \rfloor$.

\begin{table}[H]
\centering
    \begin{tabular}{||c | c||} 
        \hline
        Communication Model & Optimal Resilience \\
        \hline
        \hline
        Synchronous & $\lfloor \frac{n-1}{2} \rfloor$ \\ 
        \hline
        Asynchronous & $\lfloor \frac{n-1}{3} \rfloor$ \\
        \hline
        Semi-synchronous & $\lfloor \frac{n-1}{3} \rfloor$ \\
        \hline
    \end{tabular}
\vspace{2ex}
\caption{Optimal resilience of Byzantine consensus protocols under different communication models}
\label{table:optimal-resilience}
\vspace{-4mm}
\end{table}

These optimal resilience thresholds are based on the assumption that nodes in the system are equivalent such that they have the same voting power.
In an open system like Bitcoin \cite{Nakamoto2008} where nodes can join and leave freely, making such an assumption is prone to the Sybil attack \cite{Douceur2002} where an attacker can create identities in the system cheaply and gain more voting power.
Once the voting power of the attacker exceeds the optimal resilience, it can break the safety property of the system.
In this scenario, the voting power of nodes should depend on some resource which cannot be easily replicated. Section 2.2 discusses how to prevent Sybil attacks under an open environment in details.

\subsection{Proof-of-work Protocols}
Proof of work is originally proposed to deter spammers and discourage junk mail \cite{DN1993}.
Bitcoin is the first cryptocurrency that adopted PoW to prevent Sybil attacks \cite{Nakamoto2008}.
The main idea is that to generate a new block, a node is required to solve a computationally intensive cryptographic puzzle.
The puzzle is designed in such a way that the solution cannot be found faster than by brute-force search.
To solve the puzzle, a node needs to find a $nonce$.
When combining the $nonce$ with the $payload$ in a block, such as the hash of previous block and the hash of the root of the merkle tree, as the input to a public known hash function $H(\cdot)$ (such as SHA-256), the output should be less than a small number $D$ which is a difficulty parameter \cite{Nakamoto2008}.

The voting power in the PoW system is essentially the computation power owned by the node.
In addition, Bitcoin will only reward the block proposers of the blocks which are on the longest chain.
For a Bitcoin miner to increase its portion of blocks on the longest chain, it needs to invest more computation power into solving the puzzles.
This reward-distribution scheme instills competition among the miners and aggravates energy consumption.
Nowadays, the total power consumption by Bitcoin is about 135 TWh a year, comparable to the annual power consumption of Sweden \cite{BitcoinEnergy}.

Although Bitcoin is designed with the vision to be a decentralized system, it becomes more centralized as the total computation power in Bitcoin increases \cite{GBE+2018,CHL2021}.
The same phenomenon happens to Ethereum \cite{wood2014ethereum} as well, which is another popular PoW blockchain.
About 90\% of mining power is controlled by only 16 distinct mining entity in Bitcoin and only 11 distinct mining entity in Ethereum.
One possible explanation is that most small miners are risk-averse, which means their utility is a strictly concave function of the reward.
It has been shown by \cite{SBB+2016,LS2019,CHL2021} that the reward scheme used by Bitcoin and Ethereum is not collusion-proof in the sense that miners are incentivized to form mining pools to reduce reward variance.
Another potential reason is that the cost of mining (such as electricity cost) is different among the miners and \cite{AW} shows that this asymmetric cost can lead to centralized mining.

\subsection{Finality.}
One of the problems of blockchains is that forking may happen due to network delays and the randomness from the selection mechanisms.
For example, multiple Bitcoin miners may solve the puzzles for the blocks at the same height around the same time and nodes may receive different blocks at the same height.
This leads to a divergent view of the order and the content of the blocks.

Bitcoin \cite{Nakamoto2008} and many other permissionless blockchains use the longest-chain rule to resolve forks.
The longest-chain rule requires the nodes to follow the longest chain when facing forks and break ties in favour of the fork which was discovered first.
Protocols adopting the longest-chain rule usually ask nodes to confirm a block when there are $k$ more blocks after it, where $k$ is a safety parameter.
A larger $k$ means a higher probability that the block will not be reverted, but also a longer confirmation latency.
Another problem caused by the forks and the longest-chain rule is selfish mining \cite{ES2014}.
When a node possesses more than $\frac{1}{3}$ of the voting power, it is incentivized to hide the block created by itself to maximize utility.

By contrast, committee-based consensus protocols \cite{GHM+2017,BKM2019} using certificates of votes can provide nearly instant finality of a new block.
As soon as a node receives enough votes for a block, it can mark the block as finalized since no other blocks at the same height will also receive enough votes.
In this case, forks will never happen or will only happen with a negligible probability, and the protocols will not suffer from selfish mining.
