# Supplementary material for: IRS: An Incentive-compatible Reward Scheme for Algorand
Source: arXiv:2302.11178 source file (2023-02-22)
Supplement: Supplementary file 2 [file 11-appendix-referral-proofs.tex]

\section{Proof of \reflemm{lemm:expected-rewards}}
\label{app:referral-proofs}
Using the same techniques in the proof of \reflemm{lemm:expected-utility}, we can write:
\begin{align*}
\EX_{a,\theta}&[R_i(a^*(\theta), \theta) \given \theta_{i,0} = 0] = \; s_c \; \EX_{\theta}\left[\sum_{k=1}^{K(\theta)} R_i(a^*(\theta), \theta) \given[\Big] \theta_{i,0} = 0\right] \\
= & \; s_c \; \sum_{\ell=1}^{\kmax} \sum_{k=1}^{\ell} \EP(K(\theta) = \ell) \; \EX_{\theta}\left[R_i(a^*(\theta), \theta) \given \theta_{i,0} = 0, K(\theta) = \ell\right].
\end{align*}
For the remaining of the proof, we focus on case (I) in the definition of $R_i(a, \theta)$.
The proof easily extends to other three cases.
We first consider agent $i$ with $\theta_{i,0} = 0$.
\begin{align*}
\EP(K&(\theta) = \ell) \; \EX_{\theta}\left[R_i(a^*(\theta), \theta) \given \theta_{i,0} = 0, K(\theta) = \ell\right] \\
= & \; (R^{b}(k) / n_{rs}) \sum_{j \in N_i} \EP(K(\theta) = \ell) \; \EP(\theta_{j,k} \le p_c, a^*_j(\theta) \in \{C,M\} \given \theta_{i,0} = 0, K(\theta) = \ell) \\
& + R^c(k) \; \EP(K(\theta) = \ell) \; \EP( \theta_{i,k} \le p_c \given \theta_{i,0} = 0, K(\theta) = \ell) \\
& + (R^{r}(k) / \vert \hat{N}_i \vert) \sum_{j \in \hat{N}_i} \EP(K(\theta) = \ell) \; \EP(\theta_{j,k} \le p_c, a^*_j(\theta) = C \given \theta_{i,0} = 0, K(\theta) = \ell) \\
= & \; (R^{b}(k) / n_{rs}) \sum_{j \in N_i} \EP(K(\theta) = \ell) \; \EP(\theta_{j,k} \le p_c \given K(\theta) = \ell) \\
& + R^c(k) \; \EP(K(\theta) = \ell) \; \EP( \theta_{i,k} \le p_c \given K(\theta) = \ell) \\
& + (R^{r}(k) / \vert \hat{N}_i \vert) \sum_{j \in \hat{N}_i} \EP(K(\theta) = \ell) \; \EP(\theta_{j,k} \le p_c, \theta_{j,0} = 0 \given K(\theta) = \ell) \\
= & \; (R^{b}(k) / n_{rs}) \sum_{j \in N_i} \EP(\theta_{j,k} \le p_c) \; \EP(K(\theta) = \ell \given \theta_{j,k} \le p_c) \\
& + R^c(k) \; \EP(\theta_{i,k} \le p_c) \; \EP(K(\theta) = \ell \given \theta_{i,k} \le p_c) \\
& + (R^{r}(k) / \vert \hat{N}_i \vert) \sum_{j \in \hat{N}_i} \EP(\theta_{j,k} \le p_c, \theta_{j,0} = 0) \; \EP(K(\theta) = \ell \given \theta_{j,k} \le p_c, \theta_{j,0} = 0) \\
= & \; (R^{b}(k) / n_{rs}) \sum_{j \in N_i} p_c \; \EP(K(\theta) = \ell) \\
& + R^c(k) \; p_c \; \EP(K(\theta) = \ell) \\
& + (R^{r}(k) / \vert \hat{N}_i \vert) \sum_{j \in \hat{N}_i} p_c \; (1-p_b) \; \EP(K(\theta) = \ell) \\
= & \; (R^b(k) \; p_c + R^c(k) \; p_c + R^r(k) \; p_c \; (1 - p_b)) \; \EP(K(\theta) = \ell) .
\end{align*}
The second equality holds because there is no dependency between any two elements of $\theta$.
Moreover, given the definition of $a^*$, $a^*_j(\theta) \in \{C,M\}$ for all $\theta$, and $a^*_j(\theta) = C$ if and only if $\theta_{j,0} = 0$.
The third equality follows from the Bayes' rule.
The forth equality hold due to \refequ{equ:asymptotic-independence} and the fact that $K(\theta) = \ell$ is independent from $\theta_{i,k} \le p_c$ for all $i$.

Next, we consider agent $i$ with $\theta_{i,0} = 1$.
When agent $i$ is corrupted by the adversary, it strictly prefers action $M$.
We can write the conditional expectation of agent $i$'s reward for $(s_i, s^*_{-i})$ as:
\begin{align*}
\EX_{a,\theta}&[R_i(a^*(\theta), \theta) \given \theta_{i,0} = 1] = \; \EX_{\theta}\left[\sum_{k=1}^{K(\theta)} R_i(a^*(\theta), \theta) \given[\Big] \theta_{i,0} = 1\right] \\
= & \; \sum_{\ell=1}^{\kmax} \sum_{k=1}^{\ell} \EP(K(\theta) = \ell) \; \EX_{\theta}\left[R_i(a^*(\theta), \theta) \given \theta_{i,0} = 1, K(\theta) = \ell\right] .
\end{align*}
Given the definition of $R_i(a, \theta)$, we have the following for case (I).
The derivation of equations is analogous to the above case when $\theta_{i,0} = 0$.
\begin{align*}
\EP(K&(\theta) = \ell) \; \EX_{\theta}\left[R_i(a^*(\theta), \theta) \given \theta_{i,0} = 1, K(\theta) = \ell\right] \\
= & \; (R^{b}(k) / n_{rs}) \sum_{j \in N_i} \EP(K(\theta) = \ell) \; \EP(\theta_{j,k} \le p_c, a^*_j(\theta) = M \given \theta_{i,0} = 1, K(\theta) = \ell) \\
& + R^c(k) \; \EP(K(\theta) = \ell) \; \EP( \theta_{i,k} \le p_c \given \theta_{i,0} = 1, K(\theta) = \ell) \\
& + (R^{r}(k) / \vert \hat{N}_i \vert) \sum_{j \in \hat{N}_i} \EP(K(\theta) = \ell) \; \EP(\theta_{i,k} \le p_c \given \theta_{i,0} = 1, K(\theta) = \ell) \\
= & \; (R^{b}(k) / n_{rs}) \sum_{j \in N_i} \EP(K(\theta) = \ell) \; \EP(\theta_{j,k} \le p_c, \theta_{j,k}=1 \given K(\theta) = \ell) \\
& + R^c(k) \; \EP(K(\theta) = \ell) \; \EP( \theta_{i,k} \le p_c \given K(\theta) = \ell) \\
& + (R^{r}(k) / \vert \hat{N}_i \vert) \sum_{j \in \hat{N}_i} \EP(K(\theta) = \ell) \; \EP(\theta_{i,k} \le p_c \given K(\theta) = \ell) \\
= & \; (R^{b}(k) / n_{rs}) \sum_{j \in N_i} \EP(K(\theta_{j,k} \le p_c, \theta_{j,k}=1) \; \EP(K(\theta) = \ell \given \theta_{j,k} \le p_c, \theta_{j,k}=1) \\
& + R^c(k) \; \EP(\theta_{i,k} \le p_c) \; \EP(K(\theta) = \ell \given \theta_{i,k} \le p_c) \\
& + (R^{r}(k) / \vert \hat{N}_i \vert) \sum_{j \in \hat{N}_i} \EP(\theta_{i,k} \le p_c) \; \EP(K(\theta) = \ell \given \theta_{i,k} \le p_c) \\
= & \; (R^{b}(k) / n_{rs}) \sum_{j \in N_i} p_c \; p_b \; \EP(K(\theta) = \ell) \\
& + R^c(k) \; p_c \; \EP(K(\theta) = \ell) \\
& + (R^{r}(k) / \vert \hat{N}_i \vert) \sum_{j \in \hat{N}_i} p_c \; \EP(K(\theta) = \ell) \\
= & \; (R^b(k) \; p_c \; p_b + R^c(k) \; p_c + R^r(k) \; p_c) \; \EP(K(\theta) = \ell) .
\end{align*}
